# Supplementary material for: Scalable PAC-Bayesian Meta-Learning via the PAC-Optimal Hyper-Posterior: From Theory to Practice
Source: arXiv:2211.07206 source file (2023-12-22)
Supplement: Supplementary file 1 [file supplement.tex]

\newpage

\beginsupplement

\appendix

\section*{Appendix}

\section{Proofs and Derivations}

\subsection{Bounding $\Psi(\beta, k)$ in Theorem~\ref{theorem:alquier_pac_bound}}
\label{appendix:bounding_psi}

\paragraph{Bounded loss function}
When the loss function is bounded, that is, $l:\calF \times \calZ \rightarrow [a, b]$, we can use Hoeffding's lemma to bound $\Psi(\beta, n)$. In particular, we define the random variable $l_j = \calL(h, \calD) - l(h,z_j) \in [a-b, b-a]$ and write 
\begin{align} 
\begin{split} 
\Psi(\beta, k) = & \ln \E \exp \left(\frac{\beta}{k} \sum_{j=1}^k l_j \right) = \sum_{j=1}^k \ln \E \exp \left(\frac{\beta}{k} l_j \right) \\
\leq &  \sum_{j=1}^k \ln \E \exp \left(\frac{\beta^2 4 (b-a)^2 }{8 k^2}\right) = \frac{\beta^2 (b-a)^2 }{2 k}
\end{split}
\end{align}

\paragraph{Sub-gamma loss}
A loss function $l$ is considered \emph{sub-gamma} with variance factor $s^2$ and scale parameter $c$, under a prior $\pi$ and data distribution $\calD$, if it can be described by a sub-gamma random variable $V := \calL(h, \calD) - l(h,z)$, that is, its moment generating function is upper bounded by that of a Gamma distribution $\Gamma(s, c)$:
\begin{equation*}
\ln  \E_{f \sim \pi} \E_{z \sim \calD} \left[ e^{\lambda V} \right]
\leq \frac{\lambda^2 s^2}{2(1- c \lambda)} \quad \forall \lambda \in ( 0, 1 / c )
\end{equation*}
For details see \citet{Boucheron2013, germain2016pac}. We can use the sub-gamma assumption to bound $\Psi(\beta, k)$ as follows
\begin{equation}
\Psi(\beta, k) = \sum_{j=1}^k \ln \E \exp \left(\frac{\beta}{k} l_j \right) \leq   \frac{\beta^2 s^2}{2 k (1- \frac{c \beta}{k})} 
\end{equation}

\paragraph{Sub-gaussian loss} A \emph{sub-gaussian} loss function with variance $s^2$ can be considered as limit case of the previously discussed sub-gamma assumption when $c \rightarrow 0^+$. As direct consequence, $\Psi(\beta, n)$ can be bounded by
\begin{equation}
\Psi(\beta, k) \leq \frac{\beta^2 s^2}{2 k} 
\end{equation}

\subsection{Proof of Lemma~\ref{lemma:optimal_gibbs_posterior}} 
To avoid measure theoretic arguments, we only provide a proof for the case when $A = \{a_1, ..., a_K \}$ is a countable set. For the general case, see \citet{zhang2006information} and \citet{catoni2007pac}. When $A$ is countable, we can express probability densities as categorical distributions, i.e. $\rho(a_k) = \rho_k$ and $\pi(a_k) = \pi_k ~ \forall k $  where $\sum_{k=1}^K \rho_k = \sum_{k=1}^K \pi_k = 1$, $\pi_k, \rho_k > 0$.

This allows us to write the task of finding $\rho^*$ as constraint optimization problem:
\begin{equation}
\argmin_{\rho \in [0, \infty)^K } J(\rho) = \argmin_{\rho \in [0, \infty)^K } \sum_{k=1}^K \rho_k \left( \beta g(a_k)+ \ln \frac{\rho_k}{\pi_k} \right)  \quad \text{s.t.} \quad \sum_{k=1}^K \rho_k = 1
\end{equation}

The respective Lagrangian reads as
\begin{equation}
\calL(\rho, \lambda) = \sum_{k=1}^K \rho_k \left( \beta g(a_k)+ \ln \frac{\rho_k}{\pi_k} \right) - \lambda \left( \sum_{k=1}^K \rho_k - 1 \right)
\end{equation}
with the respective partial derivatives:
\begin{align}
\frac{\partial \calL}{\partial q_k} &= \beta g(a_k) + \ln \frac{\rho_k}{\pi_k} - \lambda = 0 \qquad k = 1, ..., K \label{eq:partial_wrt_qk}\\ 
\frac{\partial \calL}{\partial \lambda} &= \sum_{k=1}^K \rho_k - 1 = 0 \label{eq:partial_wrt_lagrange_multimlpier}
\end{align}

From (\ref{eq:partial_wrt_qk}) we get that
\begin{equation} \label{eq:rhok_with_multiplier}
\rho_k = \pi_k e^{\lambda - \beta g(a_k)} 
\end{equation}
which we insert in (\ref{eq:partial_wrt_lagrange_multimlpier}) to identify the Lagrange multiplier as log-partition function:
\begin{equation} \label{eq:log_partition_fn}
\lambda = - \ln \sum_{k=1}^K \pi_k e^{ - \beta g(a_k)} 
\end{equation}
Finally, using (\ref{eq:log_partition_fn}) in (\ref{eq:rhok_with_multiplier}) we obtain
\begin{equation}
q_k^* = \frac{\pi_k e^{- \beta g(a_k)} }{\sum_{k=1}^K \pi_k e^{ - \beta g(a_k)}}
\end{equation}
which concludes the proof. Note, that $q_k^*$ fulfills the non-negativity constraint $\rho \in [0,\infty)^K$ since $\pi_k \geq 0$. Hence, the Hessian $\nabla^2_\rho J(\rho) = \text{diag} (\rho_1^{-1}, ..., \rho_K^{-1})$ is positive semi-definite $\forall \rho \in [0,\infty)^K$ and $\rho^*$ the global minimizer of $J(\rho)$ within the $K$-dimensional probability simplex. $\hfill \Box$

%% END PROOF OF LEMMA

%%%%%%%%%%%%%%%%%%%%%%%%%%%%%%%%%%%%%%%%%%%%%%%%%%%%%%%%%%%%%%%%%%%%%%%%%%%%%%%%
\subsection{Proof of Theorem~\ref{theorem:meta-learning-bound-bounded-lossfn}}
\label{appendix:proof_theorem_meta_pac_bound}

\paragraph{Step 1 (Task specific generalization)}

First we bound the generalization error of each of the observed tasks $\tau_i=(\calD_i, m_i)$, when a learning algorithm $Q: \calM \times \calZ^{m_i} \rightarrow \calM$ which outputs a posterior distribution $Q=Q(S_i, P)$ over hypotheses $\theta$, given a prior distribution $P$ and a data set $S_i \sim \calD^{m_i}_i$ of size $m_i$.

In particular, we use Theorem~\ref{theorem:alquier_pac_bound} with the following with the following instantiations. The samples are $Z^k = S_i$ with $k := m_i$ and distribution $\calD := \calD_i$. Further, we define $f := (P, h)$ as a tuple of a prior distribution $P$ and hypothesis $h$. 
This can be understood as a two-level hypothesis, wherein $P$ constitutes a hypothesis of the meta-learning problem and $h$ a hypothesis for solving the classical machine learning task at hand. In a similar manner, we define two-level priors and posteriors, i.e. $\pi = (\calP, P)$ and $\rho = (\calQ, Q(S_i, P))$, denoting the distribution of first sampling $P$ from $\calQ$ and then $\theta$ from $Q(S_i, P)$.

Using the above definitions, the KL-divergence term can be re-written in the following way:
\begin{align*}
    KL(\rho || \pi) &= \E_{h \sim \rho} \left[ \ln \frac{\rho(h)}{\pi(h)} \right] = \E_{P \sim \calQ} \left[ \E_{h \sim Q(P, S_i)} \left[ \ln \frac{\calQ(P) Q(S_i, P)(h)}{\calP(P) P(h)}\right] \right] \\
    &= \E_{P \sim \calQ} \left[ \ln \frac{\calQ(P)}{\calP(P)}\right] + \E_{P \sim \calQ} \left[ \E_{h \sim Q(P, S_i)} \left[ \ln \frac{Q(S_i, P)(h)}{P(h)}\right] \right] \\
    &= KL(\calQ||\calP) + \E_{P \sim \calQ} \left[ KL(Q(P, S_i) || P)\right]
\end{align*}

%%%%%%%%%%%%%%%%%%%%%%%%%%%%%%%%%%%%%%%%%%%%%%%%%%%%%%%%%%%%%%%%%%%%%%%%%%%
Finally, we can bound the task specific generalization error based on Theorem~\ref{theorem:alquier_pac_bound} with $\beta := m_i$, obtaining
\begin{align} 
\begin{split}
\calL(\calQ, \calD_i) &\leq   \E_{P \sim \calQ} \E_{h \sim Q} \left[ \hat{\calL}(h, S_i) \right]  + \frac{1}{m_i} \left( KL(\calQ||\calP) + \E_{P \sim \calQ} \left[ KL(Q || P)\right] + \ln \frac{1}{\delta_i} + \Psi(m_i, m_i) \right)
\end{split} \label{eq:task-level_bound}
\end{align}
which holds over all choices of $(\calQ,Q) \in \calM(\calM(\calH)) \times \calM(\calH)$ with probability at least $1 - \delta_i$.

\paragraph{Step 2 (Task environment generalization)}

In the next step, we bound the generalization on the task-environment level. Let $\tau_i=(\calD_i, m_i) \sim \calT$ be tasks drawn i.i.d from the task-environment distribution $\calT$. We set $f := P$, $\pi := \calP$ and $\rho := \calQ$ and define the meta-level empirical loss function as $l(f, S) = \hat{\calL}(h, M) = \frac{1}{n} \sum_{i=1}^n \calL(h, D_i)$. Let denote the hyper-prior and hyper-posterior. As a result from Theorem~\ref{theorem:alquier_pac_bound} with $\beta:=n$, we obtain
\begin{align}
\calL(\calQ, \calT) \leq \hat{\calL}(\calQ, M) + \frac{1}{n} \left( D_{KL}(\calQ || \calP) + \ln \frac{1}{\delta_0} + \Psi(n,n) \right) \label{eq:meta-level_bound}
\end{align}
over all $\calQ \in \calM(\calM(\calH))$ with probability at least $\geq 1 - \delta_0$

\paragraph{Union bound}

Finally, we have to combine the results from Step 1 and 2. For that, we bound the probability of the intersection of the events in (\ref{eq:task-level_bound}) and (\ref{eq:meta-level_bound}) with a union bound argument. In particular, for any $\delta > 0$ we set $\delta_i := \frac{\delta}{2n}$ and $\delta_0 = \frac{\delta}{2}$. Further, we define $\overline{m} = \left( \frac{1}{n} \sum_{i=1}^n \frac{1}{m_i} \right)^{-1}$ as the harmonic mean of the sample sizes $m_i$. 

\begin{align}
\calL(\calQ, \calT)  \leq ~ & \hat{\calL}(\calQ, M) + \frac{1}{n} \left( D_{KL}(\calQ || \calP) + \ln \frac{2}{\delta}  +  \Psi(n,n) \right) \\
  \leq ~ & \frac{1}{n} \sum_{i=1}^n \calL(\calQ, \tau_i) +
   \frac{1}{n} \left( D_{KL}(\calQ || \calP) + \ln \frac{2}{\delta}  +  \Psi(n,n)  \right) \\
  \leq ~ & \frac{1}{n} \sum_{i=1}^n \hat{\calL}(\calQ, S_i) + \frac{1}{n} \sum_{i=1}^n \frac{1}{m_i} \left( KL(\calQ||\calP) + \E_{P \sim \calQ} \left[ KL(Q_i || P)\right] + \ln \frac{2n}{\delta} +  \Psi(m_i, m_i) \right) \\
  & +\frac{1}{n} \left( D_{KL}(\calQ || \calP) + \ln \frac{2}{\delta} +  \Psi(n,n) \right)\\
  = ~ & \hat{\calL}(\calQ, S_1, ..., S_n) + \left(\frac{1}{n} + \frac{1}{\overline{m}}\right)  KL(\calQ||\calP) + \frac{1}{n} \sum_{i=1}^n \frac{1}{m_i} \E_{P \sim \calQ} \left[ KL(Q_i || P)\right]\\
  & + \frac{1}{\overline{m}}  \ln \frac{2n}{\delta} + \frac{1}{n} \ln \frac{2}{\delta} + \frac{1}{n}  \Psi(n,n) + \frac{1}{n} \sum_{i=1}^n \frac{1}{m_i} \Psi(m_i,m_i) \\
   = ~ & \hat{\calL}(\calQ, S_1, ..., S_n) + \left(\frac{1}{n} + \frac{1}{\overline{m}}\right)  KL(\calQ||\calP) + \frac{1}{n} \sum_{i=1}^n \frac{1}{m_i} \E_{P \sim \calQ} \left[ KL(Q_i || P)\right] + C(\delta, n, \overline{m})
\end{align}

In that, we defined $C(\delta, n, \overline{m})$ as 
\begin{equation}
C(\delta, n, \overline{m}) := \frac{1}{\overline{m}}  \ln \frac{2n}{\delta} + \frac{1}{n} \ln \frac{2}{\delta} + \frac{1}{n}  \Psi(n,n) + \frac{1}{n} \sum_{i=1}^n \frac{1}{m_i} \Psi(m_i,m_i)
\end{equation}

\paragraph{Bounded loss function}
If we assume that the loss function is bounded, that is $l: \calH \times \calZ \rightarrow [a,b]$, we can use (\ref{eq:psi_bound_bounded_loss}) to bound $C(\delta, n, \overline{m})$ as follows:
\begin{align}
C(\delta, n, \overline{m}) \leq ~ & \frac{1}{\overline{m}}  \ln \frac{2n}{\delta} + \frac{1}{n} \ln \frac{2}{\delta} + \frac{1}{n}  \frac{n^2(b-a)^2}{2n} + \frac{1}{n} \sum_{i=1}^n \frac{1}{m_i} \frac{m_i^2(b-a)^2}{2m_i} \\
= ~ &  \frac{1}{\overline{m}}  \ln \frac{2n}{\delta} + \frac{1}{n} \ln \frac{2}{\delta} + (b-a)^2
\end{align}

\paragraph{Sub-gamma loss function}
If we assume that the loss function is sub-gamma with variance factor $s^2$ and scale parameter $c$, under the two-level prior $(\calP, P)$ and the data distribution $(\calT, \calD)$, we can use (\ref{eq:psi_bound_sub_gamma}) to bound $C(\delta, n, \overline{m})$ as follows:
\begin{align}
C(\delta, n, \overline{m}) \leq ~ & \frac{1}{\overline{m}}  \ln \frac{2n}{\delta} + \frac{1}{n} \ln \frac{2}{\delta} + \frac{1}{n}  \frac{n^2s^2}{2n(1-c)} + \frac{1}{n} \sum_{i=1}^n \frac{1}{m_i} \frac{m_i^2s^2}{2m_i(1-c)} \\
= ~ &  \frac{1}{\overline{m}}  \ln \frac{2n}{\delta} + \frac{1}{n} \ln \frac{2}{\delta} + \frac{s^2}{1-c}
\end{align} $\hfill \Box$

%%%%%%%%%%%%%%%%%%%%%%%%%%%%%%%%%%%%%%%%%%%%%%%%%%%%%%%%%%%%%%%%%%%%%%%%%%%%%%%%%%%%%%%%%%%%%
\subsection{PAC-Bayes Meta-Learning Bound with Marginal Likelihood}
\label{appendix:derivation_bound_marginal_likelihood}

When we choose $Q$ as optimal Gibbs posterior $Q^*_i := Q^*(S_i, P)$, it follows that 
\begin{align}
& \hat{\calL}(\calQ, S_1, ..., S_n) + \frac{1}{n} \sum_{i=1}^n \frac{1}{m_i} \E_{P \sim \calQ} \left[ KL(Q^*_i || P)\right] \\
=~& \frac{1}{n} \sum_{i=1}^n \left( \E_{P \sim \calQ} \E_{h \sim Q^*_i} \left[ \hat{\calL}(h, S_i) \right]  + \frac{1}{m_i} \left( \E_{P \sim \calQ} \left[ KL(Q^*_i || P)\right] \right) \right) \\
=~& \frac{1}{n} \sum_{i=1}^n \frac{1}{m_i} \left(\E_{P \sim \calQ} \E_{h \sim Q^*_i} \left[ m_i \hat{\calL}(h, S_i) +  \ln \frac{Q^*_i(h)}{P(h)} \right] \right) \label{eq:task_objective_in_bound} \\
=~& \frac{1}{n} \sum_{i=1}^n \frac{1}{m_i} \left(\E_{P \sim \calQ} \E_{h \sim Q^*_i} \left[ \sum_{j=1}^{m_i} l(h, z_i) +  \ln \frac{P(h) e^{- \sum_{j=1}^{m_i} l(h, z_i) }}{P(h) Z(S_i, P)} \right] \right) \\
=~& \frac{1}{n} \sum_{i=1}^n \frac{1}{m_i} \left(- \E_{P \sim \calQ} \left[ \ln Z(S_i, P)\right] \right)
\end{align}

This allows us to write the inequality in (\ref{eq:meta-learning-bound}) as 
\begin{align} \label{eq:meta_pac_bound_mll_appendix}
\calL(\calQ, \calT)  \leq ~  & - \frac{1}{n} \sum_{i=1}^n \frac{1}{m_i} \E_{P \sim \calQ} \left[\ln Z(S_i, P) \right]  + \left(\frac{1}{n} + \frac{1}{\overline{m}}\right)  KL(\calQ||\calP) + C(\delta, n, \overline{m})
\end{align}

Due to Lemma~\ref{lemma:optimal_gibbs_posterior} is the Gibbs posterior $Q^*(S_i, P)$ is the minimizer of (\ref{eq:task_objective_in_bound}), in particular
\begin{equation}
Q^*(S_i, P) = \frac{P(h)e^{- m  \hat{\calL}(h,S_i)}}{Z(S_i,P)} = \argmin_{Q \in \calM(\calH)} \E_{h \sim Q} \left[ \hat{\calL}(h, S_i) \right]  + \frac{1}{m_i} KL(Q || P) \quad \forall P \in \calM(\calH), \forall i=1, ..., n
\end{equation}

Hence, we can write
\begin{align}
\calL(\calQ, \calT)  \leq & - \frac{1}{n} \sum_{i=1}^n \frac{1}{m_i} \E_{P \sim \calQ} \left[\ln Z(S_i, P) \right]  + \left(\frac{1}{n} + \frac{1}{\overline{m}}\right)  KL(\calQ||\calP) + C(\delta, n, \overline{m}) \\
= & \frac{1}{n} \sum_{i=1}^n \E_{P \sim \calQ} \left[\min_{Q \in \calM(\calH)} \hat{\calL}(Q, S_i)  + \frac{1}{m_i}  KL(Q || P) \right] + \left(\frac{1}{n} + \frac{1}{\overline{m}}\right)  KL(\calQ||\calP) + C(\delta, n, \overline{m}) \\
\leq & \frac{1}{n} \sum_{i=1}^n \E_{P \sim \calQ} \left[\hat{\calL}(Q, S_i)  + \frac{1}{m_i}  KL(Q || P) \right] + \left(\frac{1}{n} + \frac{1}{\overline{m}}\right)  KL(\calQ||\calP) + C(\delta, n, \overline{m}) \\
= & \hat{\calL}(\calQ, S_1, ..., S_n) + \left(\frac{1}{n} + \frac{1}{\overline{m}}\right)  KL(\calQ||\calP) + \frac{1}{n} \sum_{i=1}^n \frac{1}{m_i} \E_{P \sim \calQ} \left[ KL(Q_i || P)\right] + C(\delta, n, \overline{m})
\end{align}
which proofs that bound for Gibbs optimal base learners in (\ref{eq:meta_pac_bound_mll_appendix}) and (\ref{eq:meta-level_pac_bound_with_mll}) is tighter than the bound in Theorem~\ref{theorem:meta-learning-bound-bounded-lossfn} which holds uniformly for all $Q \in \calM(\calH)$. $\hfill \Box$

\subsection{Proof of Proposition~\ref{proposition:optimal-hyper-posterior}: PAC-Optimal Hyper-Posterior}
\label{appendix:proof_optimal-hyper-posterior}

In this section we derive the hyper-posterior distribution $\calQ \in \calM(\calM(\calH))$ which, given a hyper-prior $\calP \in \calM(\calM(\calH))$ and datasets $S_1, ..., S_n$, minimizes the PAC-Bayesian meta-learning bound in (\ref{eq:meta-level_pac_bound_with_mll}). 

An objective function corresponding to (\ref{eq:meta-level_pac_bound_with_mll}) reads as
\begin{equation} \label{eq:meta-objective_with_mll}
J(\calQ) =  - \E_{\calQ} \left[ \frac{~\overline{m}}{\overline{m} + n} \sum_{i=1}^n \frac{1}{m_i} \ln Z(S_i, P) \right] + KL(\calQ||\calP) 
\end{equation}
To obtain $J(\calQ)$ omit all additive terms from (\ref{eq:meta-level_pac_bound_with_mll}) that do not depend on $\calQ$ and multiply by the scaling factor $\frac{\overline{m} n}{\overline{m} + n}$. Since the described transformations are monotone, the any minimizing distribution of $J(\calQ)$, i.e.
\begin{equation}
\calQ^* = \argmin_{\calQ \in \calM(\calM(\calH))} J(\calQ)
\end{equation}
is also the minimizer of (\ref{eq:meta-level_pac_bound_with_mll}). More importantly, $J(\calQ)$ is structurally similar as the generic minimization problem in (\ref{eq:gibbs_agrmin}). Hence, we can invoke Lemma~\ref{lemma:optimal_gibbs_posterior} with $A = \calM(\calH)$, $g(a) = - \sum_{i=1}^n \frac{1}{m_i} \ln Z(S_i, P)$, $\beta = \frac{\overline{m}}{\overline{m} + n}$, to show that the optimal hyper-posterior is
\begin{equation}
\calQ^*(P) = \frac{\calP(P) \exp \left(  \frac{\overline{m}}{\overline{m} + n} \sum_{i=1}^n \frac{1}{m_i} \ln Z(S_i, P) \right) }{Z^{II}(S_1, ..., S_n, \calP)}
\end{equation}
wherein 
\begin{align*}
& Z^{II}(S_1, ..., S_n, \calP) = \E_{P \sim \calP} \left[ \exp \left(  \frac{\overline{m}}{\overline{m} + n} \sum_{i=1}^n \frac{1}{m_i} \ln Z(S_i, P) \right)  \right]
\end{align*} $\hfill \Box$

Technically, this concludes the proof of Proposition~\ref{proposition:optimal-hyper-posterior}. However, we want to remark the following interesting result:

If we choose $\calQ = \calQ^*$, the PAC-Bayes bound in (\ref{eq:meta-level_pac_bound_with_mll}) can be expressed in terms of the meta-level partition function $Z^{II}$, that is
\begin{align}
\calL(\calQ, \calT)  &\leq - \frac{\overline{m} + n}{\overline{m} n} \ln Z^{II}(S_1, ..., S_n, \calP) + C(\delta, n, \overline{m}) \label{eq:pac_bound_z2}
\end{align}
We omit a detailed derivation of (\ref{eq:pac_bound_z2}) since it is similar to the one in Appendix~\ref{appendix:derivation_bound_marginal_likelihood}.

\subsection{Poof Equivalence Variational Inference and Minimization of PAC-Bayes Meta-Learning Bound}
\label{appendix:proof_eqivalence_vi_pac_bound}

\begin{align} 
\tilde{\calQ} & = \argmin_{\calQ \in \calF} ~ KL(\calQ || \calQ^*) \\ 
& = \argmin_{\calQ \in \calF} ~ \E_{P \sim \calQ}  \left[ \ln \calQ(P) - \ln \calQ^*(P)\right] \\
& =  \argmin_{\calQ \in \calF} ~ \E_{P \sim \calQ}  \left[ \ln \calQ(P) - \ln \calP(P) -  \left(  \frac{\overline{m}}{\overline{m} + n} \sum_{i=1}^n \frac{1}{m_i} \ln Z(S_i, P) \right) + \ln Z^{II}(S_1, ..., S_n, \calP) \right] \\
& =  \argmin_{\calQ \in \calF}  ~ KL(\calQ || \calP) - \frac{\overline{m}}{\overline{m} + n} \sum_{i=1}^n \frac{1}{m_i} \E_{P \sim \calQ}  \left[  \ln Z(S_i, P)  \right] \label{eq:proof_eqivalence_vi_pac_bound_step3} \\ 
& =  \argmin_{\calQ \in \calF}  ~ - \frac{1}{n} \sum_{i=1}^n \frac{1}{m_i} \E_{P \sim \calQ}  \left[  \ln Z(S_i, P)  \right] + \left(\frac{1}{n} + \frac{1}{\overline{m}}\right) KL(\calQ || \calP)\label{eq:proof_eqivalence_vi_pac_bound_step4}
\end{align}
In that, we multiplied (\ref{eq:proof_eqivalence_vi_pac_bound_step3}) with  $\left(\frac{1}{n} + \frac{1}{\overline{m}}\right)$ to obtain (\ref{eq:proof_eqivalence_vi_pac_bound_step4}). Now it is straightforward to see that (\ref{eq:proof_eqivalence_vi_pac_bound_step4}) is the same as the meta-learning PAC-Bayes bound in (\ref{eq:meta-level_pac_bound_with_mll}) up to the constant $C(\delta, n, \overline{m})$. Hence, we can conclude that variational inference w.r.t. $\calQ^*$ is equivalent to minimizing (\ref{eq:meta-level_pac_bound_with_mll}) over the same variational family $\calF$.

%%%%%%%%%%%%%%%%%%%%%%%%%%%%%%%%%%%%%%%%%%%%%%%%%%%%%%%%%%%%%%%%%%%%%%%%%%%%%%%%%%%
%%%%%%%%%%%%%%%%%%%%%%%%%%%%%%%%%%%%%%%%%%%%%%%%%%%%%%%%%%%%%%%%%%%%%%%%%%%%%%%%%%
\section{Hierarchical Variational Bayes Perspective}

Hierarchical Bayes setup after \citet{amit2017meta}:

\begin{itemize}
\item $S_i$ is independent of hyper-parameter $\psi$, i.e. $p(S_i| w_i, \psi) = p(S_i| w_i)$
\item Given $w_i$, the samples $S_i = \{z_1, ..., z_{m_i}\}$ are independent, i.e. $p(S_i,w_i) = \prod_{z \in S_i} p(z|w_i)$
\item Known likelihood function $p(z|w_i)$
\item Parametric prior distribution over $w_i$ conditioned on $\psi$, $p(w_i|\psi)$
\end{itemize}

The posterior over the latent variables can be written as
\begin{align}
p(\psi, w_1, ..., w_n|S_1, ..., S_n) = p(\psi|S_1, ..., S_n) \prod_{i=1}^n p(w_i|\psi, S_i)
\end{align}

Obtaining the exact posterior is intractable. An approximate posterior can be obtained using variational inference with the following family of distributions,
\begin{equation}
q(\psi, w_1, ..., w_n) = \calQ_\theta(\psi) \prod_{i=1}^n Q_{\phi_i}(w_i)
\end{equation}
where the variational parameters can be obtained through
\begin{equation}
\argmin_{\theta, \phi_1, ..., \phi_n} KL \left( q(\theta, \phi_1, ..., \phi_n) || p(\phi, w_1, ..., w_n|S_1, ..., S_n) \right)
\end{equation}

This optimization problem can be reformulated as

\begin{equation} \label{eq:vi_hierarchical_bayes}
\argmin_{\theta, \phi_1, ..., \phi_n} \E_{\phi \sim \calQ_\theta} \sum_{i=1}^n 
\left[ - \E_{w_i \sim Q_{\phi_i}} \left[ \ln p(S_i|w_i) \right]  + KL(Q_{\phi_i} || p(w_i|\psi)) \right] +  KL(\calQ_{\theta} || \calP) 
\end{equation}

If $Q_i = Q^*_i:= \frac{p(w_i|\psi) e^{\ln p(S_i|w_i)}}{Z(\phi, S_i)}$ is the optimal Gibbs posterior (in this case same as Bayesian Posterior) and $Z(\psi, S_i) = p(S_i|\psi) = \int p(w|\psi) p(S_i|w) dw$ the marginal likelihood, then (\ref{eq:vi_hierarchical_bayes}) can be re-written as

\begin{align}
& \E_{\phi \sim \calQ} \sum_{i=1}^n 
\left[\E_{w_i \sim Q^*} \left[ - \ln p(S_i|w_i) + \ln \frac{p(w_i|\psi) p(S_i|w_i)}{p(w_i|\psi) Z(\psi, S_i)} \right]  \right]\\ & +   KL(\calQ || \calP) \\
= ~ & \E_{\phi \sim \calQ} \sum_{i=1}^n \left[ - \ln Z(\psi, S_i)  \right] +  KL(\calQ || \calP)  \label{eq:level2_hierarchical_bayes_obj}
\end{align}

In turn, the distribution $\calQ$ that minimizes (\ref{eq:level2_hierarchical_bayes_obj}) is the level-II Gibbs posterior $\calQ^*(\psi) = \frac{\calP(\psi) e^{ \sum_i \ln Z(\psi, S_i)}}{Z^{II}(S_1, ..., S_n)}$ where $Z^{II}(S_1, ..., S_n) = p(S_1, ..., S_n) = \int \calP(\psi) \prod_i Z(\psi, S_i)  d \psi$.

If we set $\calQ=\calQ*$, the objective in (\ref{eq:level2_hierarchical_bayes_obj}) coincides with the level-II log marginal likelihood, i.e.

\begin{align}
&  \E_{\phi \sim \calQ} \left[ - \sum_{i=1}^n 
 \ln Z(\psi, S_i)  \right] +  KL(\calQ || \calP) \\
= ~ & \E_{\phi \sim \calQ} \left[ - \sum_{i=1}^n 
 \ln Z(\psi, S_i) + \ln   \frac{\calP(\psi) e^{ \sum_i \ln Z(\psi, S_i)}}{\calP(\psi) Z^{II}(S_1, ..., S_n)} \right] \\
 = ~ & - \ln Z^{II}(S_1, ..., S_n)
\end{align}
