# Supplementary material for: Scalable PAC-Bayesian Meta-Learning via the PAC-Optimal Hyper-Posterior: From Theory to Practice
Source: arXiv:2211.07206 source file (2023-12-22)
Supplement: Supplementary file 3 [file supplement_playground.tex]

\section{Revised Proof of Bounding the CGFs}
    Finally, we aim to bound the random quantity $\frac{1}{\gamma} \Upsilon^{\rom{1}}(\gamma) +  \frac{1}{\lambda} \Upsilon^\rom{2}(\lambda)$. Note that the randomness of $\Upsilon^{\rom{1}}(\gamma)$ is governed by the random data points $z_{i,j}$ sampled i.i.d.\ from the respective data distribution $\calD_i$, while $\Upsilon^\rom{2}(\lambda)$ is governed by random tasks sampled from the environment $\calT$. 
    
    First, we factor out $\sqrt{n}$ from $\gamma$ and $\lambda$, obtaining
    \begin{equation} \label{eq:factor_out_sqrt_n}
    \frac{1}{\gamma} \Upsilon^{\rom{1}}(\gamma) +  \frac{1}{\lambda} \Upsilon^\rom{2}(\lambda) = \frac{1}{\sqrt{n}} \left( \frac{\sqrt{n}}{\gamma} \Upsilon^{\rom{1}}(\gamma) +  \frac{\sqrt{n}}{\lambda} \Upsilon^\rom{2}(\lambda) \right)
    \end{equation}
    Next, we proceed by bounding the inner part on the RHS, i.e., $\frac{\sqrt{n}}{\gamma} \Upsilon^{\rom{1}}(\gamma) +  \frac{\sqrt{n}}{\lambda} \Upsilon^\rom{2}(\lambda)$. Using Markov's inequality, we have 
    \begin{equation}
    e^{\frac{\sqrt{n}}{\gamma} \Upsilon^{\rom{1}}(\gamma) +  \frac{\sqrt{n}}{\lambda} \Upsilon^\rom{2}(\lambda)}  \leq  \frac{\E \left[ e^{ \frac{\sqrt{n}}{\gamma} \Upsilon^{\rom{1}}(\gamma) +  \frac{\sqrt{n}}{\lambda} \Upsilon^\rom{2}(\lambda)} \right]}{\delta}
    \end{equation}
    and thus
    \begin{equation} \label{eq:high_prob_bound_generic}
     \frac{\sqrt{n}}{\gamma} \Upsilon^{\rom{1}}(\gamma) +  \frac{\sqrt{n}}{\lambda} \Upsilon^\rom{2}(\lambda) \leq \log \E \left[ e^{ \frac{\sqrt{n}}{\gamma} \Upsilon^{\rom{1}}(\gamma) +  \frac{\sqrt{n}}{\lambda} \Upsilon^\rom{2}(\lambda)} \right] - \log \delta
\end{equation}
with probability at least $1-\delta$. Next, we bound the expectation, i.e., 

\begin{align} \label{eq:dskjfkjsdfb}
\E \left[ e^{ \frac{\sqrt{n}}{\gamma} \Upsilon^{\rom{1}}(\gamma) +  \frac{\sqrt{n}}{\lambda} \Upsilon^\rom{2}(\lambda)} \right] = ~ \E_\calT \left[ e^{\frac{\sqrt{n}}{\lambda} \Upsilon^\rom{2}(\lambda)}  ~ \E_{\calD_1} ... \E_{\calD_1} \left[  \left(e^{\Upsilon^{\rom{1}}(\gamma)}\right)^{\frac{\sqrt{n}}{\gamma} } \right] \right] ~. 
\end{align}
If $\gamma \geq \sqrt{n}$, $x \mapsto x^{\sqrt{n}/\gamma}$ is a concave function, we can obtain an upper bound on (\ref{eq:dskjfkjsdfb}) by using Jensen's inequality to move the exponent in (\ref{eq:dskjfkjsdfb}) outside the inner expectation. Further, we denote $V_i^\rom{2} := \E_{\calT} \left[ \calL (Q_i, \calD)  \right] - \calL(Q_i, \calD_i )$ as i.i.d.\ realizations of the random variable under the task distribution.  Similarly, for each $i=1, ....,n$ and $j=1,....,m$, we denote the independent realizations of $\calL(h, \calD_i) - l(h, z_{ij})$ as $V_{ij}^\rom{1}$. Hence, we can write 
\begin{align} 
    (\ref{eq:dskjfkjsdfb}) \leq & ~ \E_\calT \left[ e^{\frac{\sqrt{n}}{\lambda} \Upsilon^\rom{2}(\lambda)}  ~ \E_{\calD_1} ... \E_{\calD_1} \left[ e^{\Upsilon^{\rom{1}}(\gamma)} \right]^{\frac{\sqrt{n}}{\gamma}} \right] \\
    = & ~ \E_\calT \bigg[ \E_{\calP} \left[ e^{\frac{\lambda}{n} \sum_{i=1}^n V_i^{\rom{2}}} \right]^{\sqrt{n}/\lambda}  \cdot  \E_{\calP} \E_{P}  \E_{\calD_1} ... ~\E_{\calD_n} \left[ e^{ \frac{\gamma}{nm} \sum_{i=1}^n \sum_{j=1}^m V_{ij}^{\rom{1}}}\right]^{\sqrt{n}/\gamma}  \bigg] \\
    = & ~ \E_\calT \bigg[ \E_{\calP} \left[ \prod_{i=1}^n e^{\frac{\lambda}{n}  V_i^{\rom{2}}} \right]^{\sqrt{n}/\lambda}  \cdot \E_{\calP} \E_{P}  \E_{\calD_1} ... ~\E_{\calD_n} \left[  \prod_{i=1}^n \prod_{j=1}^m  e^{ \frac{\gamma}{nm} V_{ij}^{\rom{1}}}\right]^{\sqrt{n}/\gamma}  \bigg] ~.
\end{align}

Following the arguments of \citet[][Proof of Corollary 4]{germain2016pac}, we obtain
\begin{align} \label{eq:dskjfkljsbldkzbf}
    (\ref{eq:dskjfkjsdfb})  \leq ~ &  \E_\calT  \bigg[ \prod_{i=1}^n \E_{\calP} \left[  e^{\frac{\lambda}{n} V_i^\rom{2}} \right]^{\sqrt{n}/\lambda}   \left( \prod_{i=1}^n \prod_{j = 1}^{m} \E_{\calP} \E_{P}  \E_{\calD_i} e^{ \frac{\gamma}{nm} V_{ij}^\rom{1}}\right)^{\sqrt{n}/\gamma}  \bigg] ~.
\end{align}

\paragraph{Case I: bounded loss}
First, we bound the moment-generating function (MGF) corresponding to $\Upsilon^{\rom{1}}(\gamma)$.
If the loss function $l(h_i, z_{ij})$ is bounded in $[a,b]$, we can apply Hoeffding's lemma to the moment generating function on the right of (\ref{eq:dskjfkljsbldkzbf}), obtaining:
\begin{align}
     \E \left[ e^{ \frac{\sqrt{n}}{\gamma} \Upsilon^{\rom{1}}(\gamma) +  \frac{\sqrt{n}}{\lambda} \Upsilon^\rom{2}(\lambda)} \right]  \leq ~ & 
    \E_\calT \bigg[ \E_{\calP} \left[ \prod_{i=1}^n e^{\frac{\lambda}{n} V_i^\rom{2}} \right]^{\sqrt{n}/\lambda}  \left( \prod_{i=1}^n \prod_{j = 1}^{m} e^{\frac{\gamma^2  (b-a)^2}{8 n^2 m^2}} \right)^{\sqrt{n}/\gamma} \bigg] \\
     = ~ & \E_\calT \bigg[ \E_{\calP} \left[ \prod_{i=1}^n e^{\frac{\lambda}{n} V_i^\rom{2}} \right]^{\sqrt{n}/\lambda}  \bigg]  ~ e^{\frac{\gamma  (b-a)^2}{8 \sqrt{n} m}}
\end{align}
Crucially, the upper bound $e^{\frac{\gamma  (b-a)^2}{8 \sqrt{n} m}} \geq \E_{\calD_1} ... \E_{\calD_1} \left[  \left(e^{\Upsilon^{\rom{1}}(\gamma)}\right)^{\frac{\sqrt{n}}{\gamma} } \right]$ no longer depends on the tasks which are sampled from $\calT$ which allows us to move it outside the expectation under $\calT$.
In the second step, we follow analogous steps to bound the MGF corresponding to $\Upsilon^\rom{2}(\lambda)$. Again, assuming that $\lambda > \sqrt{n}$, we use Jensen's inequality to move the exponent outside of the outer expectation and follow the arguments of \citet[][Proof of Corollary 4]{germain2016pac} to obtain
\begin{align}
     \E \left[ e^{ \frac{\sqrt{n}}{\gamma} \Upsilon^{\rom{1}}(\gamma) +  \frac{\sqrt{n}}{\lambda} \Upsilon^\rom{2}(\lambda)} \right]  \leq ~ & e^{\frac{\gamma  (b-a)^2}{8 \sqrt{n} m}}  \left[ \prod_{i=1}^n \E_\calT \E_{\calP}  e^{\frac{\lambda}{n} V_i^\rom{2}} \right]^{\sqrt{n}/\lambda} ~.
\end{align}
From the boundedness of the loss together with Hoeffding's inequality, it follows that
\begin{align}
     \E \left[ e^{ \frac{\sqrt{n}}{\gamma} \Upsilon^{\rom{1}}(\gamma) +  \frac{\sqrt{n}}{\lambda} \Upsilon^\rom{2}(\lambda)} \right]  \leq ~ & e^{\frac{\gamma (b-a)^2}{8 \sqrt{n} m} + \frac{\lambda (b-a)^2}{8 \sqrt{n} }} \label{eq:kjdnkjnsdf}
\end{align}
Finally, we insert (\ref{eq:kjdnkjnsdf}) into (\ref{eq:high_prob_bound_generic}) and set $\gamma = n \beta$ to obtain that
\begin{align}
\frac{1}{\gamma} \Upsilon^{\rom{1}}(\gamma) +  \frac{1}{\lambda} \Upsilon^\rom{2}(\lambda)
\leq  \left( \frac{\beta}{8  m} + \frac{\lambda}{8 n} \right)  (b-a)^2 - \frac{1}{\sqrt{n}} \ln \delta
\end{align}
with probability at least $1-\delta$ which concludes our high-probability bound on the CGFs in case of a bounded loss.

\paragraph{Case II: sub-gamma loss} First, we bound the moment-generating function (MGF) corresponding to $\Upsilon^{\rom{1}}(\gamma)$. If the loss is sub-gamma with variance factor $s_{\rom{1}}^2$ and scale parameter $c_{\rom{1}}$ under the two-level prior and any data distribution $\calD$ in the support of $\calT$, i.e., 
\begin{equation}
    \E_{P \sim \calP} \E_{h \sim P}  \E_{z \sim \calD} \left[ e^{\nu (\calL(\calD, h) - l(h, z)) } \right] \leq \exp \left( \frac{\nu^2 s_{\rom{1}}^2}{2(1- \nu c_{\rom{2}})} \right) ~~ \forall ~ \nu \in (0, 1 / c_{\rom{1}})
\end{equation}
then, with $\nu := \gamma / (nm)$, we have that, if $\gamma < \frac{mn}{c_{\rom{1}}}$,
\begin{align}
    \E \left[ e^{ \frac{\sqrt{n}}{\gamma} \Upsilon^{\rom{1}}(\gamma) +  \frac{\sqrt{n}}{\lambda} \Upsilon^\rom{2}(\lambda)} \right] 
     & \leq \E_\calT  \bigg[ \prod_{i=1}^n \E_{\calP} \left[  e^{\frac{\lambda}{n} V_i^\rom{2}} \right]^{\sqrt{n}/\lambda}   \left( \prod_{i=1}^n \prod_{j = 1}^{m} \exp \left( \frac{\gamma^2 s_{\rom{1}}^2}{2 n^2 m^2(1-\frac{c_{\rom{1}}  \gamma}{nm})} \right) \right)^{\sqrt{n}/\gamma}  \bigg] \\
     & = \prod_{i=1}^n \E_\calT \E_{\calP} \left[  e^{\frac{\lambda}{n} V_i^\rom{2}} \right]^{\sqrt{n}/\lambda}   \exp \left( \frac{\gamma s_{\rom{1}}^2}{2 \sqrt{n}  m (1- \frac{ c_{\rom{1}} \gamma}{nm})} \right) \label{eq:dksjfbkjsdfsk}
\end{align}
Second, we bound the remaining moment-generating function (MGF) corresponding to $\Upsilon^{\rom{2}}(\lambda)$. For that, we use the assumption that the random variable $V_i^\rom{2} := \E_{\calT} \left[ \calL (Q_i, \calD)  \right] - \calL(Q_i, \calD_i )$ is sub-gamma with variance factor $s_{\rom{2}}^2$ and scale parameter $c_{\rom{2}}$ under the hyper-prior $\calP$ and the task distribution $\calT$. That is, its moment generating function can be bounded by that of a Gamma distribution $\Gamma(s_{\rom{2}}^2, c_{\rom{2}})$:
\begin{equation}
 \E_{(\calD, S) \sim \calT} \E_{P \sim \calP} \left[  e^{\kappa  \E_{(D,S)  \sim \calT} \left[ \calL (Q(P, S), \calD) \right] - \calL (Q(P, S), \calD )}\right] \leq   \exp \left(\frac{\kappa^2 s_{\rom{2}}^2}{2(1- c_{\rom{2}} \kappa)} \right) ~ \forall \kappa \in ( 0, 1 / c_{\rom{2}} ) ~.
\end{equation}
Using the sub-gamma assumption with $\kappa := \lambda / n$, we can further bound (\ref{eq:dskjfkjsdfb}) as:
\begin{equation}
     \E \left[ e^{ \frac{\sqrt{n}}{\gamma} \Upsilon^{\rom{1}}(\gamma) +  \frac{\sqrt{n}}{\lambda} \Upsilon^\rom{2}(\lambda)} \right]  \leq \exp \left( \frac{\lambda s^2_{\rom{2}}}{2 \sqrt{n} (1 - \frac{\lambda c_{\rom{2}}}{n})} \right)   \exp \left( \frac{\gamma s_{\rom{1}}^2}{2 \sqrt{n}  m (1- \frac{ c_{\rom{1}} \gamma}{nm})} \right) ~; \label{eq:kjndf2832ksdjcjsd}
\end{equation}
under the condition that $\lambda < \frac{n}{c_{\rom{2}}}$.

Finally, we insert (\ref{eq:kjndf2832ksdjcjsd}) into (\ref{eq:high_prob_bound_generic}) and set $\gamma = n \beta$ to obtain that
\begin{align}
\frac{1}{\gamma} \Upsilon^{\rom{1}}(\gamma) +  \frac{1}{\lambda} \Upsilon^\rom{2}(\lambda)
\leq  \frac{\beta s_{\rom{1}}^2}{2  m (1- \frac{ c_{\rom{1}} \beta}{m})} + \frac{\lambda s^2_{\rom{2}}}{2 n (1 - \frac{\lambda c_{\rom{2}}}{n})} - \frac{1}{\sqrt{n}} \log \delta
\end{align}
with probability at least $1-\delta$ which concludes our high-probability bound on the CGFs in the case of sub-gamma tail assumptions.

%%%%%%%%%%%%%%%%%%%%%%%%%%%%%%%%%%%%%%%%%%%%%%%

% \subsection{Bounding the CGFs separately}
% \lemma{}
% \begin{equation} \label{eq:factor_out_sqrt_n}
% \frac{1}{\gamma} \Upsilon^{\rom{1}}(\gamma) +  \frac{1}{\lambda} \Upsilon^\rom{2}(\lambda) = \frac{1}{\sqrt{n}} \left( \frac{\sqrt{n}}{\gamma} \Upsilon^{\rom{1}}(\gamma) +  \frac{\sqrt{n}}{\lambda} \Upsilon^\rom{2}(\lambda) \right)
% \end{equation}

% By the independence of the samples, the boundedness of $l \in [a, b]$ and Hoeffding's lemma, we can bound the MGF as follows:
% \begin{align}
% & \E_{\calD_1}, ..., \E_{\calD_n} \E_{\calP} \E_{h \sim P} \left[ e^{  \frac{\gamma}{n} \sum_{i=1}^n \calL(h, \calD_i) - \hat{\calL}(h, S_i)}  \right] \\
% = & \E_{\calP} \E_{h \sim P} \E_{\calD_1}, ..., \E_{\calD_n} \left[ \prod_{i}^n \prod_{i}^{m_i} e^{ \frac{\gamma}{nm_i} (\calL(h, \calD_i) - l(h, z_{ij}) )} \right] \\
% = &  \prod_{i=1}^n \prod_{j=1}^{m_i} \E_{z_{ij} \sim \calD_i} \left[ e^{ \frac{\gamma}{nm_i} (\calL(h, \calD_i) - l(h, z_{ij}) )} \right]  \\
% \leq & \prod_{i=1}^n \prod_{j=1}^{m_i}  e^{ \frac{\gamma^2}{n^2 m_i^2} \frac{(b-a)^2}{8}} \\
% = & e^{ \frac{\gamma^2}{n m} \frac{(b-a)^2}{8}} ~.
% \end{align}

% Using Markov's inequality, we have with probability at least $1-\delta$ that
% \begin{align}
% &  \frac{1}{\gamma} \ln \E_{\calP} \E_{h \sim P} \left[ e^{  \frac{\gamma}{n} \sum_{i=1}^n \calL(h, \calD_i) - \hat{\calL}(h, S_i)}  \right] \\
% \leq &  \frac{\gamma}{n m} \frac{(b-a)^2}{8} - \frac{1}{\gamma} \ln(\delta)
% \end{align}
